# Supplementary material for: Gen3DEval: Using vLLMs for Automatic Evaluation of Generated 3D Objects
Source: arXiv:2504.08125 source file (2025-04-10)
Supplement: Supplementary file 1 [file supp_imenc_comp_fig3.tex]

\begin{figure*}
\vspace{-1.cm}
\begin{center}
\includegraphics[width=1.\linewidth]{figures/supp_imenc_comp3.pdf}
\end{center}
\vspace{-1.5cm}
\caption{\textbf{Qualitative result from ablation study on different input image embeddings.} This image shows an advantage of \shortmethod using CLIP combined with DinoV2 compared to  standalone CLIP embeddings.}

\label{fig:supp_imenc_comp3}
\end{figure*}
